# Supplementary material for: Graph Neural Reasoning for 2-Quantified Boolean Formula Solvers
Source: arXiv:1904.12084 source file (2019-04-27)
Supplement: Supplementary file 1 [file supple_20_main.tex]

% The obvious difference between SAT and 2QBF is that in 2QBF the literals are
% quantified by $\forall$ or $\exists$. We propose our GNN embedding
% architectures for 2QBF formulae, based on the known embedding of SAT
% \citep{DBLP:journals/corr/abs-1802-03685}, but uses
% different embedding matrices and NN modules for the $\forall$- and
% $\exists$-quantifed literals.

% The simplest form of embedding (Model 1) is given below. 
\section{All GNN-embedding Architectures}

We use subscript symbols
  $\forall$ to denote all $\forall$-quantified literals,
  $\exists$ to denote all $\exists$-quantified literals,
  $L$ to denote all literals, and $C$ to denote all clauses. 
  We use notations
$\text{Emb}_{X}$ to denote embeddings of $X$, where $X$ can be subscript
$\forall$, $\exists$, $L$, or $C$. We use notations
$\text{Emb}_{\neg X}$ to denote embedding of the negations of $X$ ($\forall$, $\exists$, or $L$), which is part of
$\text{Emb}_{X}$ but at different indices. We use notations
$\text{Msg}_{X \to Y}$ to denote messages from $X$ to $Y$. We also use notations
$\mathcal{M}_{X}$ to denote MLPs that generate messages from the embeddings of $X$, notations
$\mathcal{M}_{X \to Y}$ to denote MLPs that generate messages from the embeddings of $X$ for $Y$, notations
$\mathcal{L}_{X}$ to denote LSTMs that update embeddings of $X$ given incoming messages, and notations
$\mathcal{L}_{X \leftarrow Y}$ to denote LSTMs that update embeddings of $X$ given incoming messages from $Y$. We also use notations
$\mathbb{E}_{X}$ to denote adjacency matrix of $X$ ($\forall$, $\exists$, or $C$) and clauses, notations
$X \cdot Y$ to denote matrix multiplication of $X$ and $Y$, notations
$[X, Y]$ to denote matrix concatenation of $X$ and $Y$, and notations
$X^T$ to denote matrix transportation of $X$.

The simplest form of embedding of QBF (Model 1) is given below. 

$$\small
\ba{cl}
\textbf{Model 1:} \\ 
\text{Msg}_{\forall \to C} = \mathcal{M}_{\forall} (\text{Emb}_\forall) \\
\text{Msg}_{\exists \to C} = \mathcal{M}_{\exists} (\text{Emb}_\exists) \\
\text{Emb}_{C} = \mathcal{L}_{C} (\mathbb{E}_\forall \cdot \text{Msg}_{\forall \to C} +
                 \mathbb{E}_\exists \cdot \text{Msg}_{\exists \to C}) \\
\text{Msg}_{C \to L} = \mathcal{M}_{C} (\text{Emb}_{C}) \\
\text{Emb}_\forall = \mathcal{L}_\forall ([\mathbb{E}_\forall^T \cdot \text{Msg}_{C \to L}, \text{Emb}_{\neg \forall}]) \\
\text{Emb}_\exists = \mathcal{L}_\exists ([\mathbb{E}_\exists^T \cdot \text{Msg}_{C \to L}, \text{Emb}_{\neg \exists}]) \\
\ea
$$

In Model 2, we update the clause embedding by 2 LSTMs,
each of them take the messages from $\forall$ and $\exists$ literals separately.
% We switch the order of these 2 LSTMs in Model 3.

$$\small
\ba{cl}
\textbf{Model 2:} \\ 
\text{Msg}_{\forall \to C} = \mathcal{M}_{\forall} (\text{Emb}_\forall) \\
\text{Msg}_{\exists \to C} = \mathcal{M}_{\exists} (\text{Emb}_\exists) \\
\text{Emb}_{C} = \mathcal{L}_{C \leftarrow \forall} (\mathbb{E}_\forall \cdot \text{Msg}_{\forall \to C}) \\
\text{Emb}_{C} = \mathcal{L}_{C \leftarrow \exists} (\mathbb{E}_\exists \cdot \text{Msg}_{\exists \to C}) \\
\text{Msg}_{C \to L} = \mathcal{M}_{C} (\text{Emb}_{C}) \\
\text{Emb}_\forall = \mathcal{L}_\forall ([\mathbb{E}_\forall^T \cdot \text{Msg}_{C \to L}, \text{Emb}_{\neg \forall}]) \\
\text{Emb}_\exists = \mathcal{L}_\exists ([\mathbb{E}_\exists^T \cdot \text{Msg}_{C \to L}, \text{Emb}_{\neg \exists}]) \\
\ea
$$

% $$\small
% \ba{cl}
% \textbf{Model 2:} \\ 
% \text{Msg}_{\forall \to C} = \text{MLP}_\forall (\text{Emb}_\forall) \\
% \text{Message}_\exists = \text{MLP}_\exists (\text{Emb}_\exists) \\
% \text{Emb}_{c} = \text{LSTM}_{c\forall} (\text{EdgeMatrix}_\forall (\text{Message}_\forall)) \\
% \text{Emb}_{c} = \text{LSTM}_{c\exists} (\text{EdgeMatrix}_\exists (\text{Message}_\exists)) \\
% \text{Message}_{c} = \text{MLP}_{c} (\text{Emb}_{c}) \\
% \text{Emb}_\forall = \text{LSTM}_\forall ([\text{EdgeMatrix}_\forall^T (\text{Message}_{c}), \text{Emb}_{neg}]) \\
% \text{Emb}_\exists = \text{LSTM}_\exists ([\text{EdgeMatrix}_\exists^T (\text{Message}_{c}), \text{Emb}_{neg}]) \\
% \ea
% $$
% We can reverse the order of the two LSTM embedding updates.

We switch the order of these 2 LSTMs in Model 3.

$$\small
\ba{cl}
\textbf{Model 3:} \\ 
\text{Msg}_{\forall \to C} = \mathcal{M}_{\forall} (\text{Emb}_\forall) \\
\text{Msg}_{\exists \to C} = \mathcal{M}_{\exists} (\text{Emb}_\exists) \\
\text{Emb}_{C} = \mathcal{L}_{C \leftarrow \exists} (\mathbb{E}_\exists \cdot \text{Msg}_{\exists \to C}) \\
\text{Emb}_{C} = \mathcal{L}_{C \leftarrow \forall} (\mathbb{E}_\forall \cdot \text{Msg}_{\forall \to C}) \\
\text{Msg}_{C \to L} = \mathcal{M}_{C} (\text{Emb}_{C}) \\
\text{Emb}_\forall = \mathcal{L}_\forall ([\mathbb{E}_\forall^T \cdot \text{Msg}_{C \to L}, \text{Emb}_{\neg \forall}]) \\
\text{Emb}_\exists = \mathcal{L}_\exists ([\mathbb{E}_\exists^T \cdot \text{Msg}_{C \to L}, \text{Emb}_{\neg \exists}]) \\
\ea
$$

% $$\small
% \ba{cl}
% \textbf{Model 3:} \\ 
% \text{Message}_\forall = \text{MLP}_\forall (\text{Emb}_\forall) \\
% \text{Message}_\exists = \text{MLP}_\exists (\text{Emb}_\exists) \\
% \text{Emb}_{c} = \text{LSTM}_{c\exists} (\text{EdgeMatrix}_\exists (\text{Message}_\exists)) \\
% \text{Emb}_{c} = \text{LSTM}_{c\forall} (\text{EdgeMatrix}_\forall (\text{Message}_\forall)) \\
% \text{Message}_{c} = \text{MLP}_{c} (\text{Emb}_{c}) \\
% \text{Emb}_\forall = \text{LSTM}_\forall ([\text{EdgeMatrix}_\forall^T (\text{Message}_{c}), \text{Emb}_{neg}]) \\
% \text{Emb}_\exists = \text{LSTM}_\exists ([\text{EdgeMatrix}_\exists^T (\text{Message}_{c}), \text{Emb}_{neg}]) \\
% \ea
% $$
In Model 4 we concatenate the messages from $\forall$ and $\exists$ literals.

% Model 4 in main manuscript
$$\small
\ba{cl}
\textbf{Model 4:} \\ 
\text{Msg}_{\forall \to C} = \mathcal{M}_{\forall} (\text{Emb}_\forall) \\
\text{Msg}_{\exists \to C} = \mathcal{M}_{\exists} (\text{Emb}_\exists) \\
\text{Emb}_{C} = \mathcal{L}_{C} ([\mathbb{E}_\forall \cdot \text{Msg}_{\forall \to C},
                                   \mathbb{E}_\exists \cdot \text{Msg}_{\exists \to C}]) \\
\text{Msg}_{C \to L} = \mathcal{M}_{C} (\text{Emb}_{C}) \\
\text{Emb}_\forall = \mathcal{L}_\forall ([\mathbb{E}_\forall^T \cdot \text{Msg}_{C \to L}, \text{Emb}_{\neg \forall}]) \\
\text{Emb}_\exists = \mathcal{L}_\exists ([\mathbb{E}_\exists^T \cdot \text{Msg}_{C \to L}, \text{Emb}_{\neg \exists}]) \\
\ea
$$

% $$\small
% \ba{cl}
% \textbf{Model 4:} \\ 
% \text{Message}_\forall = \text{MLP}_\forall (\text{Emb}_\forall) \\
% \text{Message}_\exists = \text{MLP}_\exists (\text{Emb}_\exists) \\
% \text{Input}_c = [\text{EdgeMatrix}_\forall (\text{Message}_\forall),
%                   \text{EdgeMatrix}_\exists (\text{Message}_\exists)] \\
% \text{Emb}_{c} = \text{LSTM}_{c} (\text{Input}_c) \\
% \text{Message}_{c} = \text{MLP}_{c} (\text{Emb}_{c}) \\
% \text{Emb}_\forall = \text{LSTM}_\forall ([\text{EdgeMatrix}_\forall^T (\text{Message}_{c}), \text{Emb}_{neg}]) \\
% \text{Emb}_\exists = \text{LSTM}_\exists ([\text{EdgeMatrix}_\exists^T (\text{Message}_{c}), \text{Emb}_{neg}]) \\
% \ea
% $$

The performance of our GNN architectures improve greatly after we realize that
(in Model 5) we may also need to use different MLP modules to generate messages
from clauses to $\forall$ and $\exists$ literals. Note that this is also the model
we reported in the main paper, and the model we decided to use for all results reported
in main paper.

$$\small
\ba{cl}
\textbf{Model 5:} \\ 
\text{Msg}_{\forall\to C} = \mathcal{M}_\forall (\text{Emb}_\forall) \\
\text{Msg}_{\exists\to C} = \mathcal{M}_\exists (\text{Emb}_\exists) \\
\text{Emb}_{C} = \mathcal{L}_{C}([\mathbb{E}_\forall \cdot \text{Msg}_{\forall\to C},
                                  \mathbb{E}_\exists \cdot \text{Msg}_{\exists\to C}]) \\
\text{Msg}_{C\to\forall} = \mathcal{M}_{C\to\forall} (\text{Emb}_{C}) \\
\text{Msg}_{C\to\exists} = \mathcal{M}_{C\to\exists} (\text{Emb}_{C}) \\
\text{Emb}_\forall = \mathcal{L}_\forall ([\mathbb{E}_\forall^T
 \cdot \text{Msg}_{C\to\forall}, \text{Emb}_{\neg \forall}]) \\
\text{Emb}_\exists = \mathcal{L}_\exists ([\mathbb{E}_\exists^T
\cdot \text{Msg}_{C\to\exists}, \text{Emb}_{\neg \exists}]) \\
\ea
$$

We also explore the possibility (in Model 6) of having two embeddings for each clause, one
serving the $\forall$ literals and one serving the $\exists$ literals.
We need extra notations:
$\text{Emb}_{X \to Y}$ denotes embeddings of $X$ that serves $Y$.
$\mathcal{L}_{X \to Y}$ denotes LSTMs that updates embedding of $X$ that serves $Y$.

$$\small
\ba{cl}
\textbf{Model 6:} \\ 
\text{Msg}_{\forall\to C} = \mathcal{M}_\forall (\text{Emb}_\forall) \\
\text{Msg}_{\exists\to C} = \mathcal{M}_\exists (\text{Emb}_\exists) \\
\text{Emb}_{C \to \forall} = \mathcal{L}_{C \to \forall}([\mathbb{E}_\forall \cdot \text{Msg}_{\forall\to C},
                                                          \mathbb{E}_\exists \cdot \text{Msg}_{\exists\to C}]) \\
\text{Emb}_{C \to \exists} = \mathcal{L}_{C \to \exists}([\mathbb{E}_\forall \cdot \text{Msg}_{\forall\to C},
                                                          \mathbb{E}_\exists \cdot \text{Msg}_{\exists\to C}]) \\
\text{Msg}_{C\to\forall} = \mathcal{M}_{C\to\forall} (\text{Emb}_{C \to \forall}) \\
\text{Msg}_{C\to\exists} = \mathcal{M}_{C\to\exists} (\text{Emb}_{C \to \exists}) \\
\text{Emb}_\forall = \mathcal{L}_\forall ([\mathbb{E}_\forall^T
 \cdot \text{Msg}_{C\to\forall}, \text{Emb}_{\neg \forall}]) \\
\text{Emb}_\exists = \mathcal{L}_\exists ([\mathbb{E}_\exists^T
\cdot \text{Msg}_{C\to\exists}, \text{Emb}_{\neg \exists}]) \\
\ea
$$

% Model 6 in main manuscript
% $$\small
% \ba{cl}
% \textbf{Model 6:} \\
% \text{Message}_\forall = \text{MLP}_\forall (\text{Emb}_\forall) \\
% \text{Message}_\exists = \text{MLP}_\exists (\text{Emb}_\exists) \\
% \text{Input}_c = [\text{EdgeMatrix}_\forall (\text{Message}_\forall),
%                   \text{EdgeMatrix}_\exists (\text{Message}_\exists)] \\
% \text{Emb}_{c\forall} = \text{LSTM}_{c\forall} (\text{Input}_c) \\
% \text{Emb}_{c\exists} = \text{LSTM}_{c\exists} (\text{Input}_c) \\
% \text{Message}_{c\forall} = \text{MLP}_{c\forall} (\text{Emb}_{c\forall}) \\
% \text{Message}_{c\exists} = \text{MLP}_{c\exists} (\text{Emb}_{c\exists}) \\
% \text{Emb}_\forall = \text{LSTM}_\forall ([\text{EdgeMatrix}_\forall^T (\text{Message}_{c\forall}), \text{Emb}_{neg}]) \\
% \text{Emb}_\exists = \text{LSTM}_\exists ([\text{EdgeMatrix}_\exists^T (\text{Message}_{c\exists}), \text{Emb}_{neg}]) \\
% \ea
% $$

We further explore possibility (in Model 7) that our embedding scheme should
reflect a CEGAR cycle, which starts from $\forall$ variables (proposing
candidates), to clauses, to $\exists$ variables (finding counterexamples), back
to clauses, then back to $\forall$ variables. 
% In the early stage of our
% experiment, we gradually decide to focus on Model 5, as it is expressive enough
% to fit the training data, and simple enough for fast turn-out and minimal
% overfitting. Note that the mathmatical process of Model 2,3,4,6, and 7 are
% provided in supplementary manuscript instead.

$$\small
\ba{cl}
\textbf{Model 7:} \\ 
\text{Msg}_{\forall\to C} = \mathcal{M}_\forall (\text{Emb}_\forall) \\
\text{Emb}_{C \to \exists} = \mathcal{L}_{C \to \exists}(\mathbb{E}_\forall \cdot \text{Msg}_{\forall\to C}) \\
\text{Msg}_{C\to\exists} = \mathcal{M}_{C\to\exists} (\text{Emb}_{C \to \exists}) \\
\text{Emb}_\exists = \mathcal{L}_\exists ([\mathbb{E}_\exists^T
\cdot \text{Msg}_{C\to\exists}, \text{Emb}_{\neg \exists}]) \\
\\
\text{Msg}_{\exists\to C} = \mathcal{M}_\exists (\text{Emb}_\exists) \\
\text{Emb}_{C \to \forall} = \mathcal{L}_{C \to \forall}(\mathbb{E}_\exists \cdot \text{Msg}_{\exists\to C}) \\
\text{Msg}_{C\to\forall} = \mathcal{M}_{C\to\forall} (\text{Emb}_{C \to \forall}) \\
\text{Emb}_\forall = \mathcal{L}_\forall ([\mathbb{E}_\forall^T
 \cdot \text{Msg}_{C\to\forall}, \text{Emb}_{\neg \forall}]) \\
\ea
$$

% Model 7 in main manuscript
% $$\small
% \ba{cl}
% \textbf{Model 7:} \\
% \text{Message}_\forall = \text{MLP}_\forall (\text{Emb}_\forall) \\
% \text{Emb}_{c\exists} = \text{LSTM}_{c\exists} (\text{EdgeMatrix}_\forall (\text{Message}_\forall)) \\
% \text{Message}_{c\exists} = \text{MLP}_{c\exists} (\text{Emb}_{c\exists}) \\
% \text{Emb}_\exists = \text{LSTM}_\exists ([\text{EdgeMatrix}_\exists^T (\text{Message}_{c\exists}), \text{Emb}_{neg}]) \\
% \\
% \text{Message}_\exists = \text{MLP}_\exists (\text{Emb}_\exists) \\
% \text{Emb}_{c\forall} = \text{LSTM}_{c\forall} (\text{EdgeMatrix}_\exists (\text{Message}_\exists)) \\
% \text{Message}_{c\forall} = \text{MLP}_{c\forall} (\text{Emb}_{c\forall}) \\
% \text{Emb}_\forall = \text{LSTM}_\forall ([\text{EdgeMatrix}_\forall^T (\text{Message}_{c\forall}), \text{Emb}_{neg}]) \\
% \ea
% $$
% \\
% \clearpage

\section{Functions for Ranking Scores}

Function for candidate ranking scores based on hardness,
i.e. the number of models of reduced SAT formula.

\begin{python}
def n_model_2_ranking_score(n_models):
    if n_models <= 3: return 10.0 - n_models
    if n_models <= 5: return 6.0
    if n_models <= 8: return 5.0
    if n_models <= 12: return 4.0
    if n_models <= 16: return 3.0
    if n_models <= 21: return 2.0
    else: return 1.0
\end{python}

Function for candidate ranking scores in maxSAT-style,
i.e. based on the number of satisfied clauses.

\begin{python}
def n_clauses_2_ranking_score(n_clauses_list):
    n_clauses_min = min(n_clauses_list)
    return [max(1, 10 - n_clauses + n_clauses_min)
            for n_clauses in n_clauses_list]
\end{python}

Function for counterexample ranking scores based on unsatisfiability cores
and number of satisfied clauses.

\begin{python}
def unsat_core_2_ranking_score(core_index,
                               n_clauses_list):
    n_clauses_max = max(n_clauses_list)
    scores = [max(1, 8 - n_clauses_max + n_clauses)
              for n_clauses in n_clauses_list]
    scores = numpy.array(scores)
    scores[core_index] = 10
    return scores.tolist
\end{python}

Function for counterexample ranking scores in maxSAT-style,
i.e. based on the number of satisfied clauses.

\begin{python}
def n_clauses_2_ranking_score_counter(n_clauses_list):
    n_clauses_max = max(n_clauses_list)
    return [max(1, 10 - n_clauses_max + n_clauses)
            for n_clauses in n_clauses_list]
\end{python}
